# Supplementary material for: Efficient Optimal Transport Algorithm by Accelerated Gradient descent
Source: arXiv:2104.05802 source file (2021-07-19)
Supplement: Supplementary file 1 [file supp_experiments.tex]

\section{More Experiments}
In this section, we firstly show the convergent curves of $E_\lambda(\psi)$, $\langle P_\lambda, C \rangle$ and $E(\psi)$ with the metrics of squared Euclidean distance and spherical distance. Then we test the performance of the proposed algorithm under different cost functions to show that $E(\psi_\lambda)$ provides a better approximation than $\langle P_\lambda, C \rangle$ by the Sinkhorn algorithm \cite{Cuturi2013Sinkhorn}.

\begin{figure*}[]
\centering
\begin{tabular}{cc}
    \includegraphics[width=.45\linewidth]{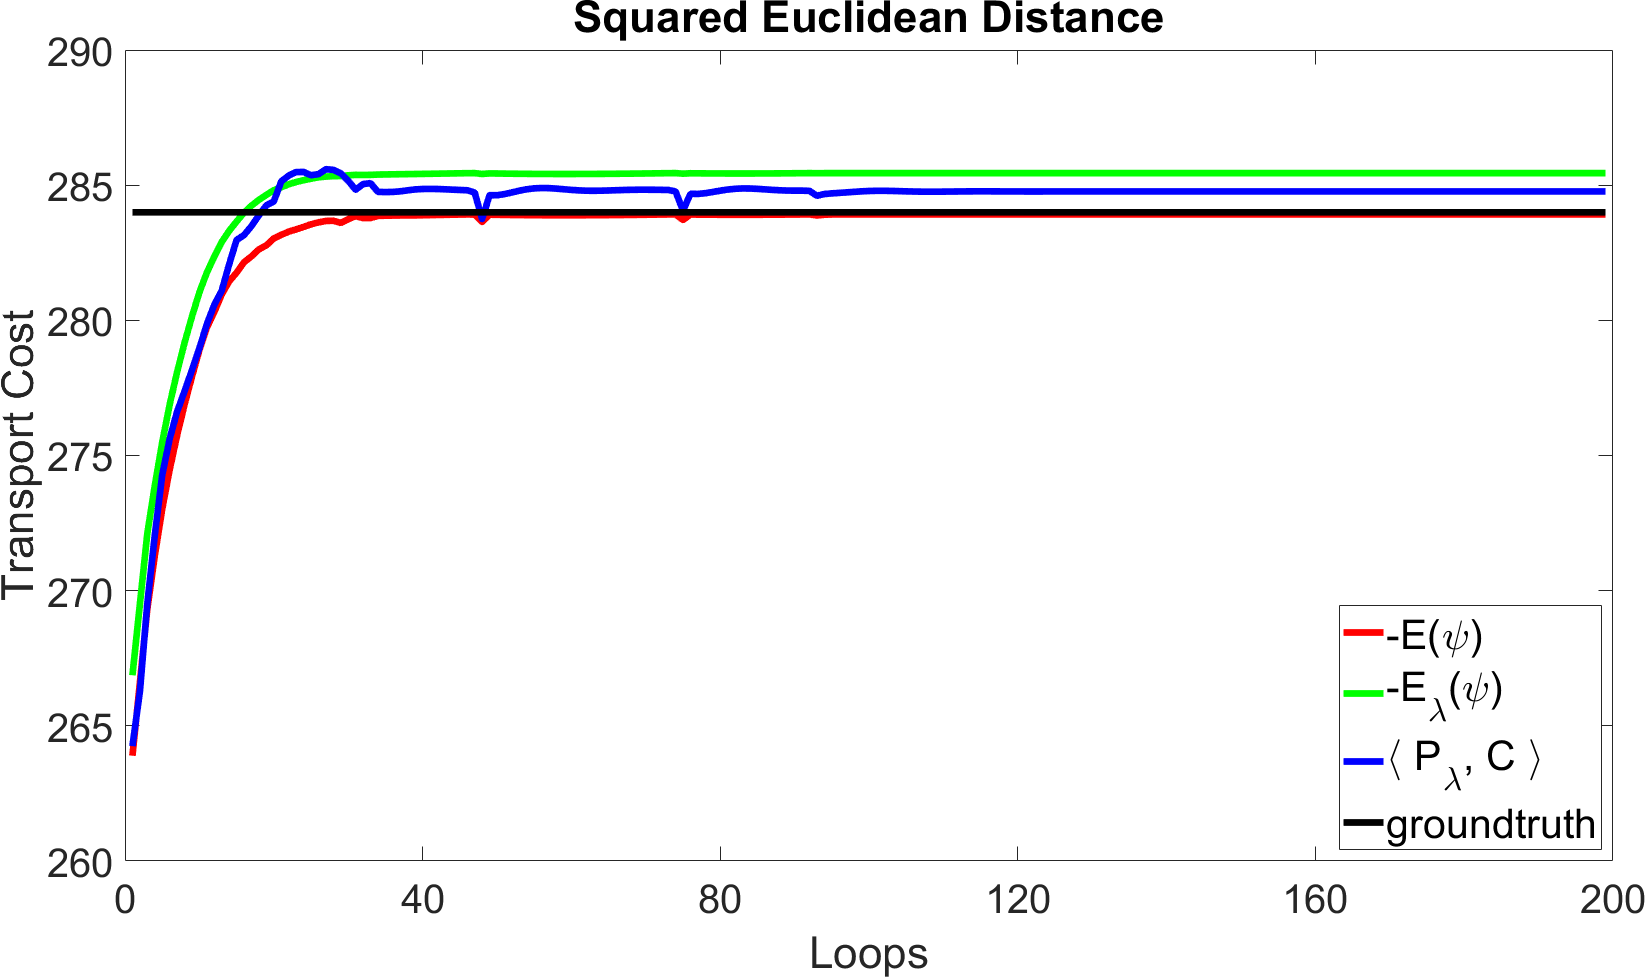} &
    \includegraphics[width=.45\linewidth]{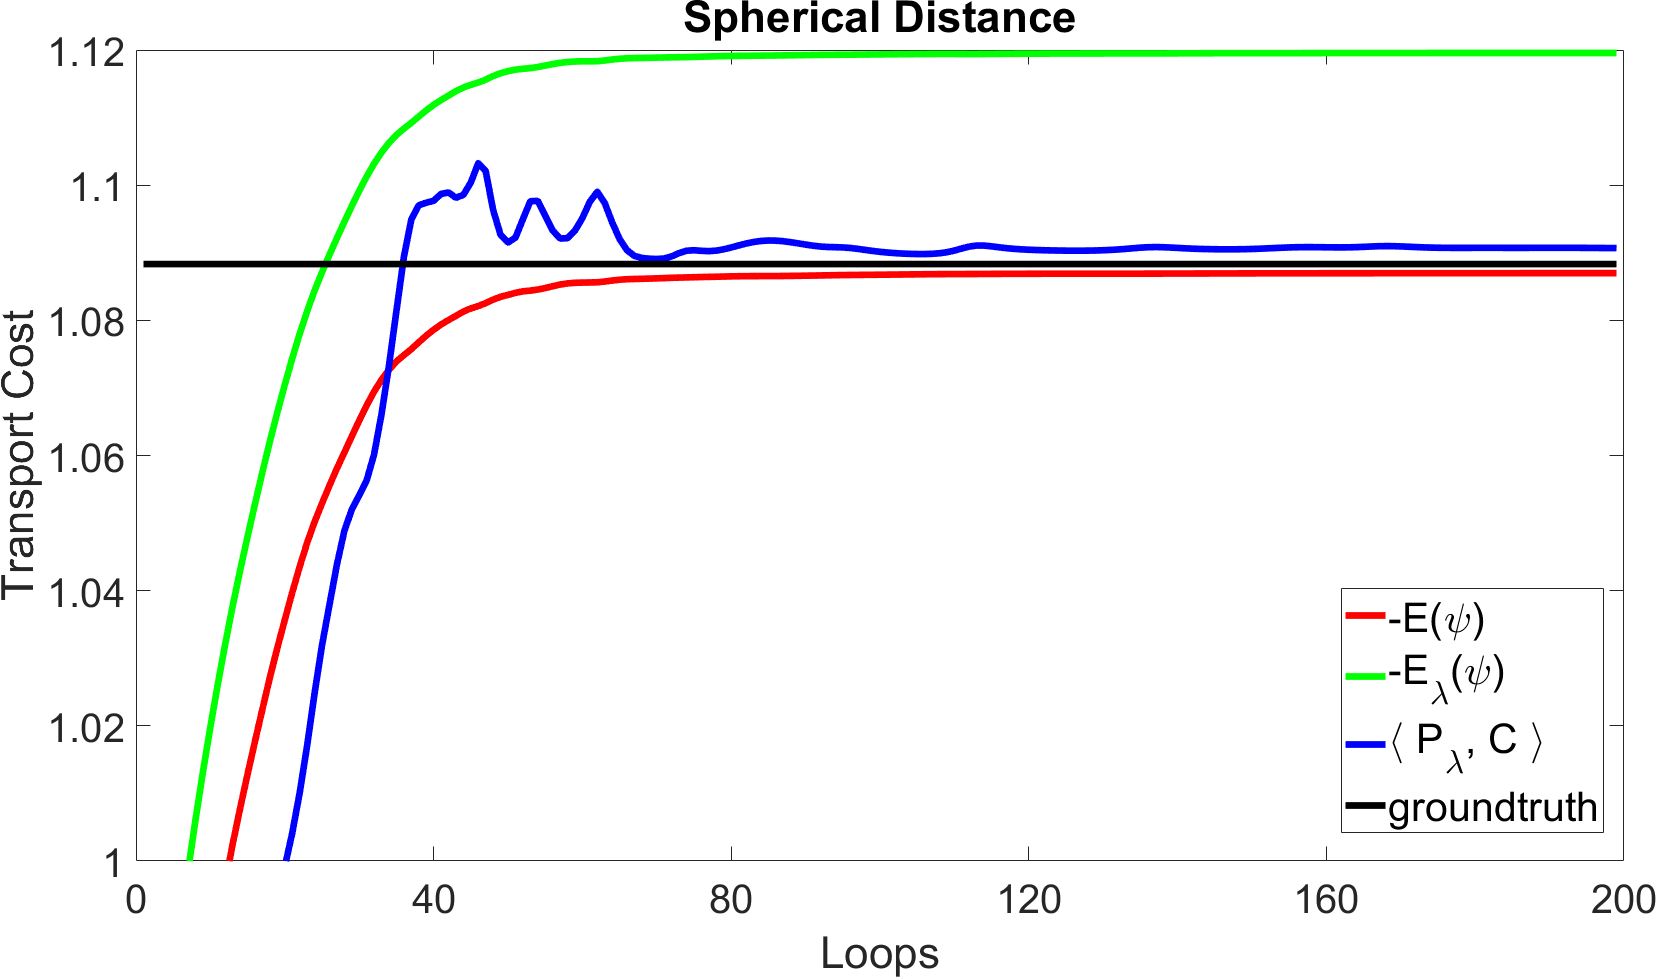}
\end{tabular}
\vspace{-3mm}
\caption{The convergent curves of $E(\psi)$, $E_\lambda(\psi)$ and $\langle P_\lambda, C\rangle$.}
    \label{fig:curves}
\end{figure*}

\begin{table*}[t]
\centering
\caption{Comparison among the OT cost (GT), the Sinkhorn result and the result of the proposed method with $T=500$ under different $P$.}
\label{tab:P_compare}
\begin{tabular}{c|ccc|cc}
\hline
P   & GT      & Sinkhorn & Ours    & |Sinkhorn-GT| & |Ours-GT| \\ \hline
1.5 & 103.33  & 103.51   & 103.27  & 0.18          & \textbf{0.06}      \\ \hline
2   & 281.7   & 282.5    & 281.6   & 0.8           & \textbf{0.1}       \\ \hline
3   & 2189.8  & 2197.1   & 2187.5  & 7.3           & \textbf{2.3}       \\ \hline
4   & 16951.4 & 17038.5  & 16932.0 & 87.1          & \textbf{19.4}      \\ \hline
\end{tabular}
\end{table*}

\subsection{More illustrations of $T$ and $\eta$}
\textbf{The Parameter $T$} The computer can only represent numbers in fixed precision. For example, if double-precision floating-point format is used in 64-bit processors, the range of the number is about $2.2251e^{-308} \sim 1.7977e^{+308}$ when using MATLAB. Based on the property 1 of the problem (\ref{eq:cpt2}), the optimal solvers of $E(\psi)$ with respect to the original cost matrix $C$ and the new matrix $C-\frac{\max(C)+\min(C)}{2}$ are the same. Thus,
to fully utilize the range of the exponential for current computer architecture and get more accurate results, we  set $C=C-\frac{\max(C)+\min(C)}{2}$. If taking no consideration of $\psi$, $\lambda$ can be as small as about $\frac{R}{600}$ in Eqn. (\ref{eqn: smooth_energy}) to keep numerical stability, namely no 'Inf' or 'NAN' output. In reality, we set $\lambda = \frac{R}{T}$ and use $T$ to control $\lambda$. Here $R=\max(C)-\min(C)$. Larger $T$ will give better approximation.

\textbf{The Parameter $\eta$} For the FISTA algorithm, the ideal fixed step size is $\eta_t=\frac{1}{\lambda_{\max}}$, where $\lambda_{\max}$ is the maximum eigenvalue of the Hessian matrix, as shown in Eqn. (\ref{eqn:Hessian}). However, accurate estimate of $\lambda_{\max}$ is hard and we only know $\lambda_{\max} \leq \frac{1}{\lambda}$, so we turn to set $\eta_t = \eta \lambda$. For one thing, if $\lambda$ is relatively large, only with small step size, the algorithm may run out of the precision range of the processor and thus get 'Inf' or 'NAN'. Thus, $\eta$ may be far less that $1$. For the other thing, we have $H\leq \frac{1}{\lambda}\max_i(\frac{\max_j K_{ij}v_j}{\mathbf{K_iv}})\leq \frac{1}{\lambda}$, we may also choose $\eta > 1$ when $\lambda$ itself is small. As a result, for different tasks, $\eta$ may change a lot.

\subsection{More experimental results}
In this experiment, we set $m=n=500$, $T=500$, and adjust $\eta$ to get the best performance of the proposed algorithm. Basically, for the squared Euclidean distance, $\eta=50$; for the spherical distance, $\eta=0.02$. In Fig. \ref{fig:curves}, we show the performance of $E(\psi)$, $E_\lambda(\psi)$ and $\langle P_\lambda, C\rangle$, where $P_\lambda$ is the approximate transport plan computed by Eqn. (\ref{eq:ot_plan}) with parameter $\lambda$. It is obvious that when the algorithm converges, we have $\langle P_\lambda^*, C\rangle \geq \langle P^*, C\rangle = - E(\psi^*) \geq - E(\psi_\lambda^*)$. Here $P_\lambda^*$ is the computed approximate OT plan given the optimizer $\psi_\lambda^*$ for $E_\lambda(\psi)$, $P^*$ and $\psi^*$ are the OT plan and optimal solver for $E(\psi)$, respectively. Though both $\langle P_\lambda^*, C\rangle$ and $-E(\psi_\lambda^*)$ approximate the optimal transport cost well, the latter performs much better.

We also explore this phenomenon with more experiments. We randomly sample $m=500$ samples from the Gaussian distribution $\mathcal{N}(3\mathbf{1}_5, \mathbf{I}_5)$ as the support of the source measure, represented by $x_i, i=1,2,\ldots,m$; and randomly sample $n=500$ samples from the Uniform distribution $Uni([-5,-4]^5)$ as the support of the target measure, denoted by $y_j,j=1,2,\ldots,n$. The source and target measures are given by $\mu=\sum_{i=1}^m \mu_i\delta(x-x_i)$ and $\nu=\sum_{j=1}^n \nu_i\delta(y-y_i)$, where both $\mu_i$s and $\nu_j$s are sampled from the uniform distribution $Uni([0,1])$ and then normalized by $\mu_i=\mu_i/\sum_{i=1}^m \mu_i$ and $\nu_j=\nu_j/\sum_{j=1}^n \nu_i$. The cost function is set as $c(x_i, y_j)=\|x_i-y_j\|^P$ with $P=1.5,2,3,4$, respectively. In Tab. \ref{tab:P_compare}, we show the OT cost given by linear programming, the Sinkhorn result and $-E(\psi_\lambda^*)$ by setting $T=500$. It is obvious that as $P$ increase, the error of the Sinkhorn result and the proposed method also increase. However, our results performs much better than Sinkhorn. This matches our analysis that Sinkhorn requires much smaller $\lambda$ to get the same error bound $\epsilon$.
Moreover, if we set $T=800$, which means that we use a much smaller $\lambda$, the proposed method still works and gets more accurate results, while the Sinkhorn will return 'NAN' due to numerical overflow. It's interesting to investigate the relationship between approximate accuracy and cost functions, and we leave this part for the future work.
